# Supplementary material for: Towards Interpretable Protein Structure Prediction with Sparse Autoencoders
Source: arXiv:2503.08764 source file (2025-03-11)
Supplement: Supplementary file 1 [file esmfold_intervention.tex]

['T1024', 'T1025', 'T1026', 'T1029', 'T1030', 'T1032', 'T1046s1', 'T1046s2', 'T1050', 'T1054', 'T1056', 'T1067', 'T1073', 'T1074', 'T1079', 'T1082', 'T1090']
