# Supplementary material for: Towards Interpretable Protein Structure Prediction with Sparse Autoencoders
Source: arXiv:2503.08764 source file (2025-03-11)
Supplement: Supplementary file 2 [file f1_eval_appendix.tex]

%% WORK IN PROGRESS 
